# Supplementary material for: IntentVizor: Towards Generic Query Guided Interactive Video Summarization
Source: arXiv:2109.14834 source file (2022-03-29)
Supplement: Supplementary file 1 [file implementation.tex]

\section*{Appendix C: Implementation Details}
Below, we will present the implementation details of our IntentVizor framework. 
As described in the main paper, our method consists two modules, i.e, intent module and summary module, both relying on Granularity-Scalable Pathway (GS-Pathway) and Ego Graph Convolutional Network (Ego-GCN). Thus, we will first describe the implementations of our proposed GS-Pathway and Ego-GCN. Then, we will further detail the intent and summary modules.
% As described in the paper, our method consists of three major modules, i.e, feature encoder, summary module and intent module. We first enumerate the implementations of the three modules before describing the training settings.
\begin{figure*}[t]
\centering
\includegraphics[trim=0 0 0 0,width=0.95\textwidth]{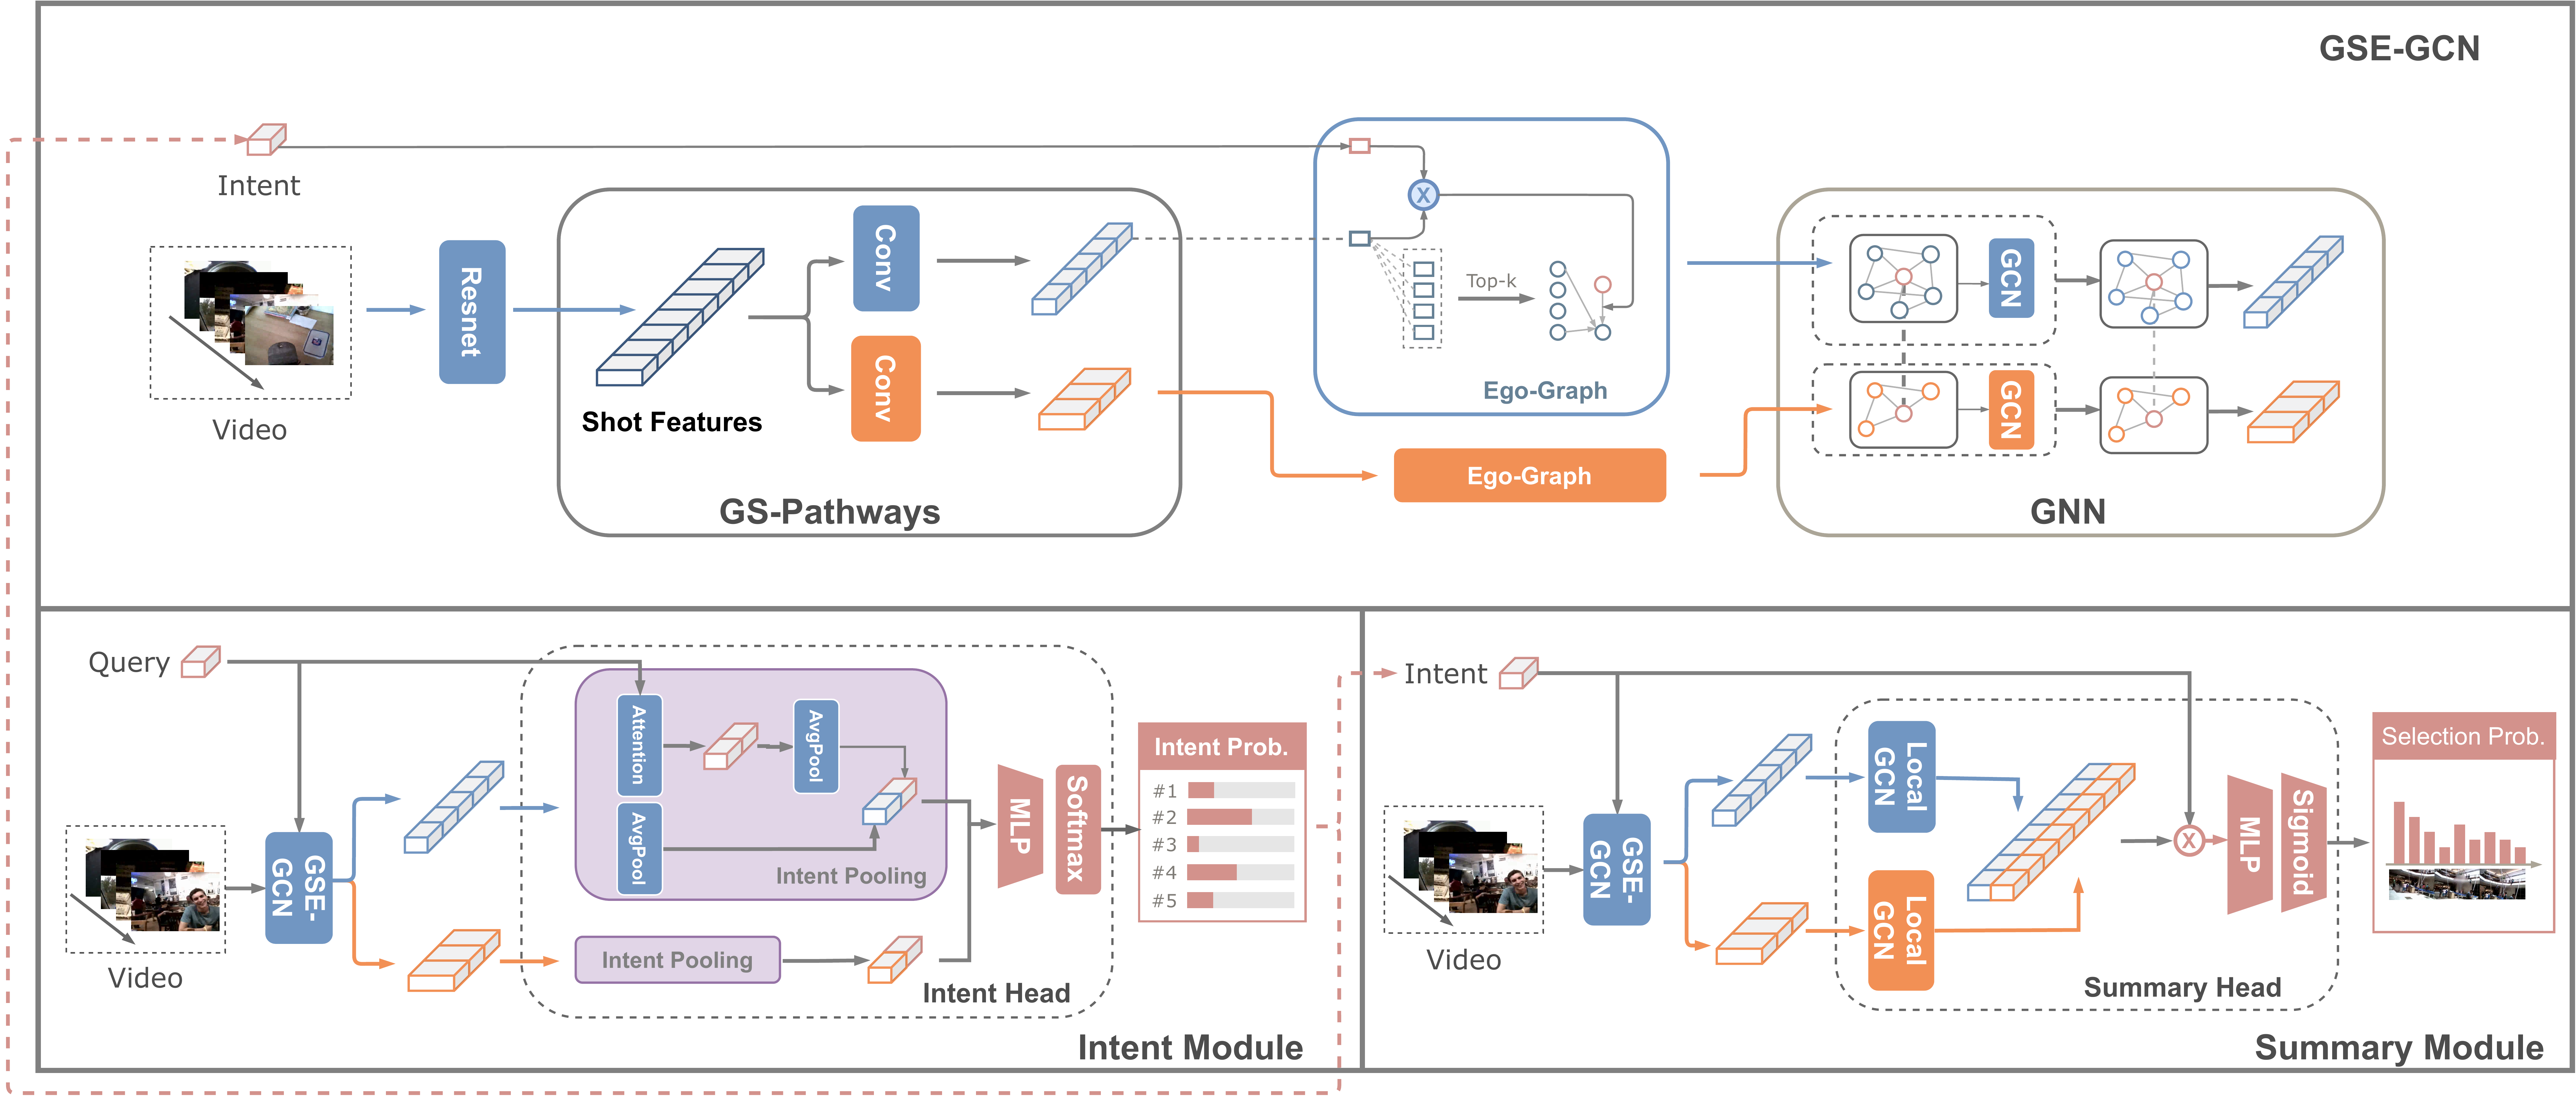} % Reduce the figure size so that it is slightly narrower than the column. Don't use precise values for figure width.This setup will avoid overfull boxes.
\caption{\textbf{GSE-GCN} exploits two notions i,e, GS-Pathway and Ego-Graph. The input video will be processed by two convolutional networks to produce two segment-level feature sequence of coarse and fine granularity. Then, each sequence will be processed to generate a Ego-Graph, where the intent/query vertex is an ego-vertex with all the video segments are connected. After feeding the graph into GCN, the two pathways will be produce the corresponding segment-level features. \textbf{Intent Head} pools the segment features into a distributed representation, which will be processed by a MLP with softmax to produce the intent probability. \textbf{Summary Head} exploits the local-GCN module to produce the shot-level features, which will be used to predict the shot selection probability.}.
\label{fig:appendix-model-overview}
\end{figure*}

\subsection*{Granularity-Scalable Pathway (GS-Pathway)}
\input{tables/slow-fast-conv}
\begin{table*}[!htbp]
\centering
%\resizebox{.95\columnwidth}{!}{
\resizebox{\textwidth}{!}{%

\begin{tabular}{lllrrrrrrrrrrrrrrrrrr}
\hline
 & \multicolumn{2}{c}{Method} & \multicolumn{3}{c}{ {   Video-1}} & \multicolumn{3}{c}{ {   Video-2}} & \multicolumn{3}{c}{ {   Video-3}} & \multicolumn{3}{c}{ {   Video-4}} & \multicolumn{3}{c}{ {   Average}} & \multicolumn{3}{c}{ {   Std Dev}} \\ \cline{2-21} 
\multirow{-2}{*}{Dataset} & \multicolumn{1}{c}{Study} & \multicolumn{1}{c}{ {   Model}} & \multicolumn{1}{c}{ {   Pre}} & \multicolumn{1}{c}{ {   Rec}} & \multicolumn{1}{c}{ {   F1}} & \multicolumn{1}{c}{ {   Pre}} & \multicolumn{1}{c}{ {   Rec}} & \multicolumn{1}{c}{ {   F1}} & \multicolumn{1}{c}{ {   Pre}} & \multicolumn{1}{c}{ {   Rec}} & \multicolumn{1}{c}{ {   F1}} & \multicolumn{1}{c}{ {   Pre}} & \multicolumn{1}{c}{ {   Rec}} & \multicolumn{1}{c}{ {   F1}} & \multicolumn{1}{c}{ {   Pre}} & \multicolumn{1}{c}{ {   Rec}} & \multicolumn{1}{c}{ {   F1}} & \multicolumn{1}{c}{ {   Pre}} & \multicolumn{1}{c}{ {   Rec}} & \multicolumn{1}{c}{ {   F1}} \\ \hline
%  & Default & Full Model & 62.19 & 45.23 & 51.27 & 50.43 & 57.81 & 53.48 & 71.03 & 51.81 & 59.56 & 27.05 & 54.04 & 35.67 & 52.68 & 52.22 & 50.00 & 19.05 & 5.28 & 10.17 \\ \cline{2-21}
 & Default & Full Model & \multicolumn{1}{r}{{62.19}} & \multicolumn{1}{r}{{45.23}} & \multicolumn{1}{r}{{51.27}} & \multicolumn{1}{r}{{50.43}} & \multicolumn{1}{r}{{57.81}} & \multicolumn{1}{r}{{53.48}} & \multicolumn{1}{r}{{73.45}} & \multicolumn{1}{r}{{53.56}} & \multicolumn{1}{r}{{61.58}} & \multicolumn{1}{r}{{28.24}} & \multicolumn{1}{r}{{56.47}} & \multicolumn{1}{r}{{37.25}} & \multicolumn{1}{r}{{{53.58}}} & \multicolumn{1}{r}{{{53.27}}} & \multicolumn{1}{r}{{{50.90}}} & 19.33	& 5.64 &	10.12 \\ \cline{2-21}
 
 &  & T+T & 53.81 & 38.89 & 44.19 & 42.31 & 49.55 & 45.82 & 60.33 & 43.97 & 50.57 & 22.84 & 45.66 & 30.11 & 44.82 & 44.52 & 42.67 & 16.44 & 4.42 & 8.80 \\ \cline{3-21}
  & Ego-GCN  & T+E & 58.24 & 42.17 & 47.89 & 43.4 & 49.76 & 46.01 & 70.06 & 50.98 & 58.66 & 24.28 & 48.63 & 32.05 & 48.995 & 47.89 & 46.15 & 19.76 & 3.93 & 10.93 \\ \cline{3-21}

 &  & E+T & 55.98 & 39.94 & 45.59 & 39.85 & 45.58 & 42.22 & 64.15 & 46.75 & 53.77 & 28.39 & 56.76 & 37.44 & 47.09 & 47.26 & 44.76 & 16.04 & 7.00 & 6.88 \\ \cline{2-21}
 
  &  & Upsampling & 56.72 & 40.65 & 46.31 & 35.61 & 40.91 & 37.8 & 39.95 & 28.68 & 33.18 & 19.89 & 39.67 & 26.21 & 38.04 & 37.48 & 35.88 & 15.14 & 5.89 & 8.43 \\ \cline{3-21}
  & Local-GCN & Transpose & 54.28 & 38.56 & 44.05 & 48.71 & 55.8 & 51.64 & 62.28 & 45.37 & 52.18 & 24.85 & 49.91 & 32.84 & 47.53 & 47.41 & 45.18  & 16.11 & 7.28 & 9.02 \\ \cline{2-21}

%  & \multirow{-2}{*}{Ego-GCN} & E+T & 58.45 & 42.3 & 48.04 & 47.9 & 54.91 & 50.8 & 66.63 & 48.51 & 55.82 & 27.73 & 55.39 & 36.57 & 50.18 & 50.28 & 47.81 & 16.81 & 6.17 & 8.15 \\ \cline{2-21}

 &  & Coarse-Only & 56.00 & 40.45 & 45.96 & 42.42 & 48.42 & 44.88 & 63.40 & 46.21 & 53.14 & 27.76 & 55.57 & 36.63 & 47.40 & 47.66 & 45.15 & 15.71 & 6.25 & 6.76 \\ \cline{3-21}
 & GS-Pathway & Fine-Only & 58.45 & 42.3 & 48.04 & 47.9 & 54.91 & 50.8 & 66.63 & 48.51 & 55.82 & 27.73 & 55.39 & 36.57 & 50.18 & 50.28 & 47.81 & 16.81 & 6.17 & 8.15 \\ \cline{3-21}
  &   & Shot Feature & 56.00 & 40.45 & 45.96 & 42.42 & 48.42 & 44.88 & 63.40 & 46.21 & 53.14 & 27.76 & 55.57 & 36.63 & 47.40 & 47.66 & 45.15 & 15.71 & 6.25 & 6.76 \\ \cline{2-21}

 &  & MiddleFusion & 56.82 & 40.97 & 46.59 & 46.27 & 53.1 & 49.1 & 69.98 & 50.32 & 57.85 & 25.05 & 50.24 & 33.08 & 49.53 & 48.66 & 46.66 & 18.98 & 5.29 & 10.26 \\  \cline{3-21}
 & \multirow{-2}{*}{Fusion Stage} & LateFusion & 54.31 & 39.2 & 44.56 & 43.89 & 50.29 & 46.53 & 65.17 & 47.51 & 54.63 & 27.4 & 54.9 & 36.17 & 47.69 & 47.98 & 45.47 & 16.08 & 6.60 & 7.58 \\ \cline{2-21}
 &  & Video Agnostic & 57.5 & 41.26 & 47 & 48.83 & 55.97 & 51.78 & 70.92 & 51.7 & 59.45 & 22.98 & 46.17 & 30.36 & 50.06 & 48.78 & 47.15 & 20.21 & 6.42 & 12.31 \\ \cline{3-21}
\multirow{-7}{*}{Textual} & \multirow{-2}{*}{Intent Module} & Video Attention & 57.29 & 41.02 & 46.75 & 44.46 & 50.98 & 47.16 & 71.87 & 52.41 & 60.26 & 23.4 & 46.99 & 30.9 & 49.26 & 47.85 & 46.27 & 20.55 & 5.10 & 12.01 \\ \cline{1-21}
 & Default & Full Model & 58.17 & 44.91 & 49.43 & 42.52 & 52.69 & 46.64 & 65.45 & 51.92 & 57.49 & 21.15 & 49.23 & 29.19 & 46.82 & 49.69 & 45.69 & 19.61 & 3.51 & 11.92 \\ \cline{2-21}
 &  & Attention Baseline & 45.01 & 33.96 & 37.71 & 38.86 & 48.01 & 41.09 & 57.7 & 48.75 & 50.66 & 18 & 41.5 & 24.75 & 39.89 & 43.06 & 38.55 & 16.57 & 6.88 & 10.71 \\ \cline{3-21} 
 & \multirow{-2}{*}{Comparative Study} & Linear Baseline & 59.24 & 45.33 & 49.75 & 21.49 & 26.71 & 23.62 & 56.09 & 44.42 & 49.22 & 14.44 & 33.1 & 19.77 & 37.82 & 37.39 & 35.59 & 23.14 & 9.04 & 16.12 \\ \cline{2-21} 
\multirow{-4}{*}{Visual} & Transferring Study & Transferring & 56.15 & 43.07 & 47.53 & 45.23 & 56.19 & 49.69 & 63.8 & 50.73 & 56.12 & 23.4 & 54.31 & 32.26 & 47.15 & 51.08 & 46.4 & 17.57 & 5.80 & 10.11 \\ \hline
\end{tabular}%

}
\caption{Full experiment result. For the models of Ego-GCN (ablation) study, T(E)+T(E) means that the model uses Transformer (Ego-GCN) as the intent module and Transformer (Ego-GCN) as the summary module respectively. For example, T+E means that the model uses Transformer as the intent module and Ego-GCN as the summary module.}
\label{tab:full-exp}
\end{table*}

Our GS-Pathway consists two pathways of different temporal granularity. Each pathway consists two convolutional layers followed by the max pooling layers respectively. We list the hyper-parameters in Table \ref{tab:slow-fast}. The processed features will be fed into the E-GCN to predict the summary and user intent.
According to Table \ref{tab:slow-fast}, the coarse pathway has a larger stride and outputs a shorter feature sequence with a length of $[\frac{T}{16}]$, where $T$ is the original video length. 
By contrast, the fine pathway has a smaller stride and outputs a longer feature sequence with a length of $[\frac{T}{4}]$. Besides, to extract the shot-level features, We employ the Resnet features provided by Xu et al. 
\cite{xiao_convolutional_2020}

\subsection*{Ego-GCN}
The Ego-Graph backbone first maps the intent/query into a space with same dimension as segment feature dimension (256 for fine pathway and 1024 for coarse pathway).We employ three GCN layers in the summary module and two layers in the intent module. Each GCN layer consists two consequential sub-layer, each of which perform one convolution operation on the constructed graph. For each GCN layer, we also add a shortcut between the input and output. Our constructed graph consists of three types of edges. There is no parameter for the temporal edge and intent-segment edge. For the semantic edge, we set the number of edges for one vertex as 8.

\subsection*{Summary Module}
Our summary module feeds the intent embedding into the GS-Pathway and Ego-GCN consequently. After that, we the processed video segment features will be fed into our summary head. 
The intent head consists of three modules, i.e, Local-GCN, dot product relevance module and MLP.

The local GCN recovers the segment-level features to the shot-level. We construct a graph for each segment where the segment vertex is connected with all shot vertices. To build the vertices, we map the segment feature and shot feature to a mutual space of 512D by a linear layer. Following Ego-GCN, we also employ temporal, semantic edges. We set the numbers of semantic edges for one shot vertex as 4 for fast pathway and 10 for slow pathway.

We employ a relevance module to compare the recovered shot-level features and the intent embedding. We first map them to a mutual space of 1024D by two linear layers respectively. Then, we perform dot product on the two generated vectors. The result will be fed into a three-lay MLP with a hidden dimension of 1024. The MLP is followed by a Sigmoid to produce the shot selection probability.

%  Local-GCN to recover the shot-level featrues from the segment-level features. Then, we relate the processed features with the intent embedding by dot product. Finally, the intent
% Our summary module consists four sub-modules described in the paper, i.e, Ego-Graph backbone, Local GCN, Relevance Module and MLP. 

% The Ego-Graph backbone first maps the intent embedding and segment features into a space with same dimension as segment feature dimension (256 for fast pathway and 1024 for slow pathway).We employ three GCN layers in the summary module. Each GCN layer consists two consequential sub-layer, each of which perform one convolution operation on the constructed graph. For each GCN layer, we also add a shortcut between the input and output. Our constructed graph consists of three types of edges. There is no parameter for the temporal edge and intent-segment edge. For the semantic edge, we set the number of edges for one vertex as 8. 

\subsection*{Intent Module}
% Intent module predicts the intent probability of each basis intent. 
The intent module predicts a weighted combination of the learned basis intent shown in Sec. 3.1.1.
We agree that the intents can be non-overlapping with the visual/textual queries when the inputted video is very different from the training data. However, the variety of queries in the dataset ensures the generalizability of the trained models.
There are two intent modules with similar structure to support the textual and visual queries respectively. 

\subsubsection*{Intent Module for Textual Query}
The intent module for textual query takes input of two query words (concepts) to predict the intent probability of the basis intents. Similar to \cite{xiao_convolutional_2020}, we employ the publicly available GLOVE word embedding \cite{pennington2014glove} to represent the query words. The inputting query words are firstly concatenated into one embedding vector(query embedding). Then, following the summary module, we employ the GSE-GCN to model the relationships between the query embedding and the segments. However, we use the query embedding as the ego vertex rather than the intent embedding. We use the same setting as we set the number of semantic edge as 8. 

Then the GSE-GCN-produced segment-level feature sequence is used by the intent head to generate the intent probability distribution. To fulfill it, the produced feature sequence is pooled temporally to obtaining a vector attending to both the video content and the query. We call the pooling module as intent pooling. The intent pooling consists two modules, i.e, attention pooling and average pooling. The average pooling performs the average pooling on the segment-level feature sequence to get a vector. By comparison, the attention pooling first inputs the queries' word embeddings as the "query" in multi-head attention module. Then, it uses the feature sequence as the "key"-"value" pair. We set the number of heads as 5. The output of the attention module has two elements corresponding to two query words. The two elements are pooled to get an average vector. Then, we concatenate the two vectors of two pathways (overall 4) and feed the concatenated vector into a three-layer MLP with a hidden dimension of 2048. Finally, we use a Softmax module to get the probability of each basis intent.

\subsubsection*{Intent Module for Visual Query}
The input of shot query intent module is the visual query consisting of $P$ shot features $\{s_1, s_2,...,s_{P}\}$. The module follows a similar structure as the text query module while it deviates in the Ego-Graph structure. 
The visual query comprises denser information with a higher feature dimension (2048D) compared with the text query (300D). Merging the visual queries together may incur a heavy loss of information. Thus, the visual query module takes the query shots as the individual vertices, and all feature vertices are connected with the queries. 
Other parameters are identical to the intent module for textual query dataset.
 
\subsection*{Baselines for the Visual Query Task}
We propose two baselines for the visual-query task in Sec. 4.2.2. Below, we will describe the implementation details for them.
\subsubsection*{Attention Baseline}
The attention baseline employs the attention mechanism to evaluate which shot is mostly related to the visual queries. The structure is similar to the QAM module (Query-focused Attention Module) in \cite{jiang_hierarchical_2019}. 
The calculated attention values are multiplied with the video shot features to produce the query-aware video features.
We stack three attention layers with the residual connection to promote the representation capability. The video features produced by the last layer is fed into a three-layer MLP to compute the selection probability for each video shot.

\subsubsection*{Transformer Baseline}
The transformer baseline employs the popular transformer structure and follows \cite{sun2019videobert}. We use the video shot and query shot as two different tokens. Then, we concatenate them and feed into a transformer encoder, which consists of three layers. Then a three-layer MLP is used to predict selection probability of each shot.
\subsection*{Training Setting}
We set the intent number as 20 and the embedding dimension as 128.
Models are trained by an Adam optimizer with a base learning rate of 1e-4 and a weight decay of 6e-5. We employ a warm-up strategy \cite{goyal2017accurate} to linearly increase the learning rate from 0 to the base learning rate in 10 epochs. After that, we reduce the learning rate to one-tenth of the previous value every twenty epochs. We set the shifted ReLU threshold as 0.05. We set the number of epochs as 120. We set the batch size as 2.

\subsection*{Fighting Overfitting}
Overfitting is a critical issue in training the deep neural networks, especially when the networks comprises a huge number of parameters. We fight the overfitting issue by both the design of network and dataset.
\begin{enumerate*}
    \item The design of the network relieves the overfitting problem. Our proposed scalable granularity can avoid overfitting by reducing the number of shots and the size of features (Sec. 3.2.1). Also, we propose to construct the graph edges based on the pre-designed heuristics to further eliminate the parameter size (Sec. 3.2.2). The standard training techniques (including early stop, momentum, gradient clip) also helps relieve the overfitting. 
    \item Though the dataset contains only four videos, each video is paired with a far larger number of different queries \cite{sharghi_query-focused_2017}. 
    % Thus, the used dataset bears both larger size and stronger diversity. 
    Also, the long videos contain a wide variety of actions/events, diversifying the dataset \cite{lee2012discovering}. 
\end{enumerate*}
