# Supplementary material for: IntentVizor: Towards Generic Query Guided Interactive Video Summarization
Source: arXiv:2109.14834 source file (2022-03-29)
Supplement: Supplementary file 2 [file prototype.tex]

\section*{Appendix B: Prototype Implementation}
\begin{figure*}[t]
\centering
\includegraphics[trim=0 0 0 95,clip, width=0.95\textwidth]{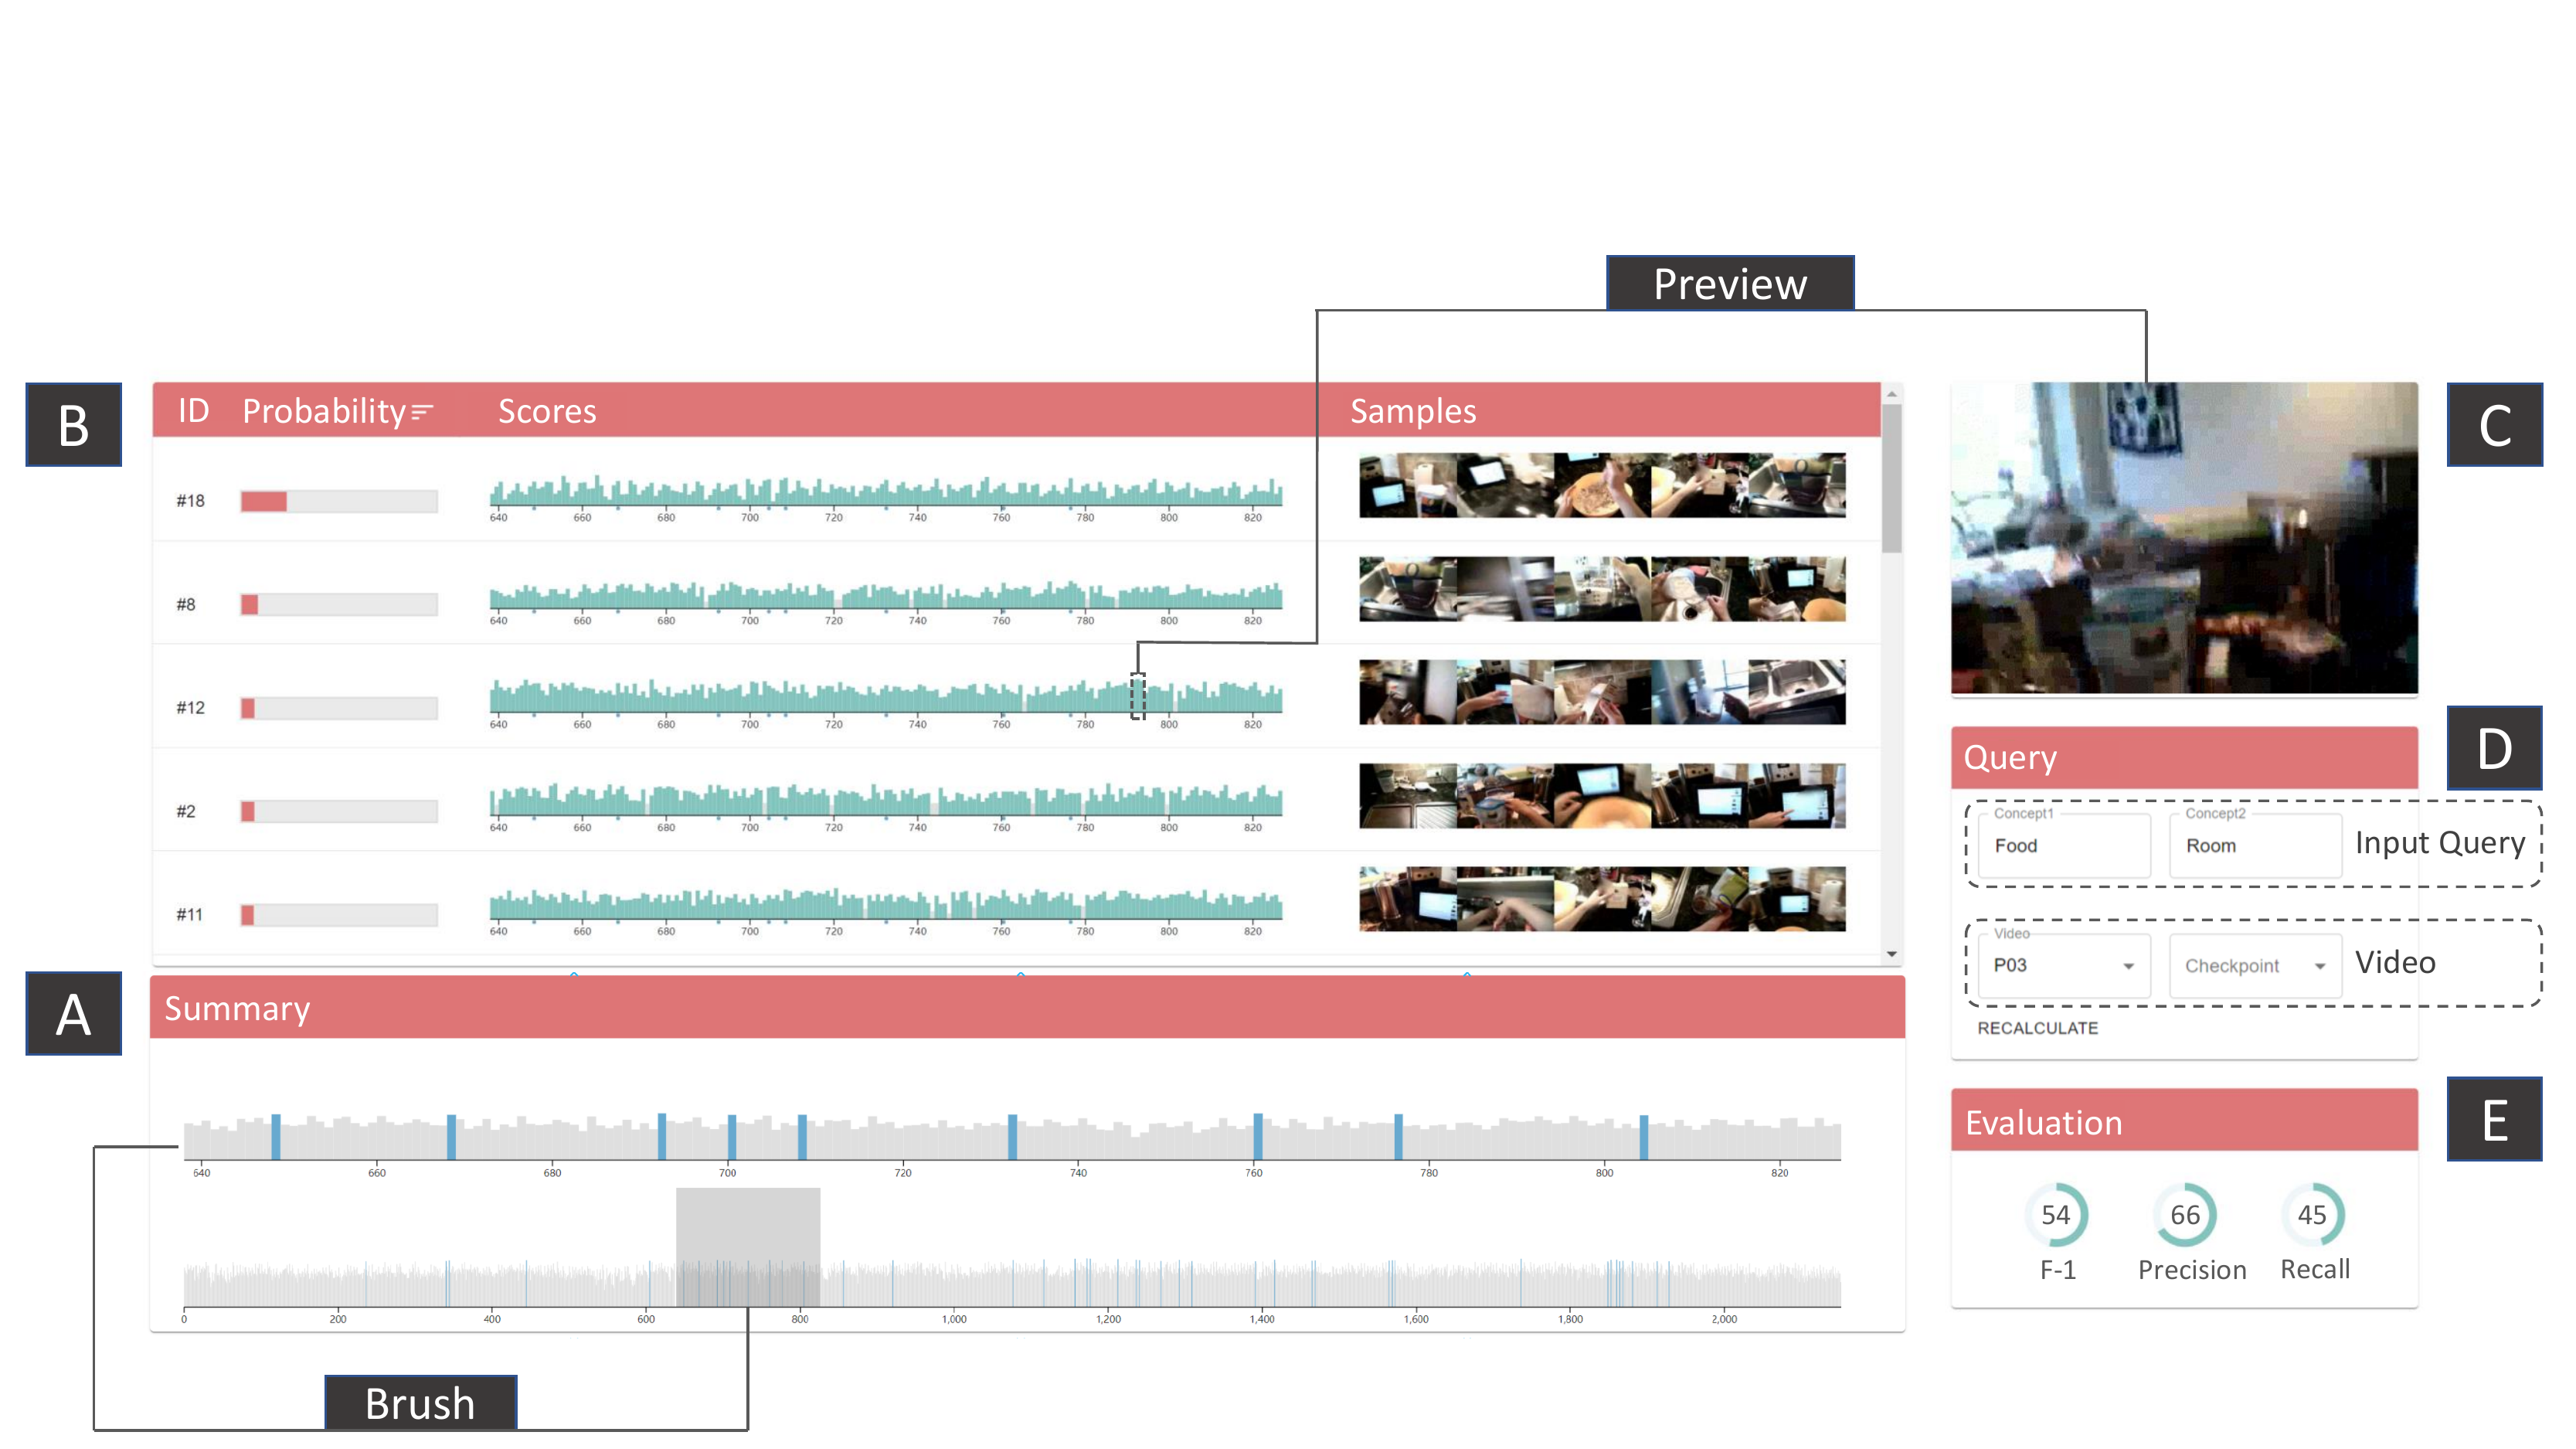} % Reduce the figure size so that it is slightly narrower than the column. Don't use precise values for figure width.This setup will avoid overfull boxes.
\caption{Prototype Overview. \textbf{A}: \textbf{Summary View} presents two temporal bar charts, which shows the overall scores and the summarized shots. The bottom bar chart shows the overview of all the shots while the top bar chart zooms into the detail decided by the brush in the bottom chart. \textbf{B}: \textbf{Intent View} list all the intents with their probability, shot scores and representative samples. The samples are selected with the highest score. \textbf{C}: \textbf{Preview View} plays a GIF of the user-hovering shot. In this case, the user hovers on the highlighted shot in intent \#12, which includes a room scenario. \textbf{D}: \textbf{Query View} allows the user to change the query and makes the model run again. \textbf{E} \textbf{Evaluation View} shows the quantitative result of the summary.}
\label{fig:appendix-prototype-overview}
\end{figure*}
In order to validate the interactivity of our proposed method, we implement a visual interface allowing the user to interact with the model. We present the implementation details below. Our prototype consists of a client-side interface and server-side
backend. The interface is built purely on browser with D3.js\cite{bostock2011d3}, React.js and Typescript. Specifically, we rely our whole interface on React.js and implement the visualization by D3.js. We implement the Restful APIs with Flask on the server-side. 
\subsection*{Client-Side Interface}
Our client interface is built with D3.js and React.js purely on Typescript. The interface consists five major components, i.e, Initial View, Summary View, Intent View,   Preview View,  Query View and Evaluation View. Below, we will first enumerate the views before presenting a user scenario.

\subsubsection*{Initial View} Initial View allows the user to select the video, textual queries and the model checkpoint. After the user submit the query, the system will automatically direct to the output of the model.

\subsubsection*{Summary View} Summary View presents the predicted summary of the corresponding video. The predicted selection probability (shot score) is visualized with a bar chart. We highlight the summary shot by the blue color. Since the videos are extremely long, as they span 3-5 hours. The user is unable to get any detail when viewing the summary ovewview. We provide a focus view on top of the summary overview. The focus view is also a bar chart while the time range is limited. The user can brush on the overview chart to control the time range in the focus view. This "focus+context" interaction style can enable the user gain the detail and overall information simultaneously. 

\subsubsection*{Intent View} Intent View lists all the intents with their probability (weight), selection probability (intent-based shot score) and representative samples. Since the representative samples are collected based on the shot probability, they can provide a visual feedback to the user and offer a impression of the specific intent. We allow the user interact with the intent probability and express their subtle intention. For example, in the use case described in our paper, the user inputs the "Food" and "Room". The user can find that intent \#18 corresponds to the food cooking when intent \# 11 focuses more on the food storage. Though the user may want to focus more on the food storage rather than food cooking. Though this type of textual query is not included in the original dataset, the user express his intention by controlling the intent probability. The case proves that our method can enable the finer-grained adjustment compared with the previous methods.

\subsubsection*{Preview View}
The Preview View shows the GIF-formatted shot. The user can hover on the shot in each intent to get its preview.

\subsubsection*{Query View} Query View is exactly same with the initial view. However, it allows the user to change the query parameters, i.e, query concepts, video and model checkpoint to re-run the model.

\subsubsection*{Evaluation View}
Evaluation view presents the quantitative evaluation of the running result. Currently we compare the user-generated summary with the ground-truth to get F-1 measure, precision and recall. We encode the result value by both the arc degree and the color. The green means the result is higher than 40\%, the yellow means the result is higher than 20\%, the red means the result is lower than 20\%. The user can adjust the intent probability, which will generate a new summary. The new summary will be automatically sent to the back-end to get the quantitative evaluation, which is then shown in this view.

\subsection*{Server-Side Backend}
\begin{table*}[!htbp]
\resizebox{\textwidth}{!}{%
\begin{tabular}{l|l|l|l|l|l}
\hline
API & Method & Parameters & Parameter Types & Response & Response Type \\ \hline
Model Preparation & GET & N/A & N/A & list of checkpoints & JSON \\ \hline
\multirow{4}{*}{Model Inference} & \multirow{4}{*}{POST} & word1 & string & \multirow{4}{*}{intent probability and shot selection probability} & \multirow{4}{*}{JSON} \\
 &  & word2 & string &  &  \\
 &  & video & string &  &  \\
 &  & checkpoint & string &  &  \\ \hline
\multirow{2}{*}{Video Shot Frame} & \multirow{2}{*}{GET} & video & string & \multirow{2}{*}{Frame Image} & \multirow{2}{*}{Image/PNG} \\
 &  & shot & integer &  &  \\ \hline
\multirow{2}{*}{Video Shot GIF} & \multirow{2}{*}{GET} & video & string & \multirow{2}{*}{Shot GIF} & \multirow{2}{*}{Image/GIF} \\
 &  & shot & integer &  &  \\ \hline
\multirow{2}{*}{Quantitative Evaluation} & \multirow{2}{*}{POST} & video & string & \multirow{2}{*}{F1, Precision and Recall} & \multirow{2}{*}{JSON} \\
 &  & summary & Array\textless{}integer\textgreater{} &  &  \\ \hline
\end{tabular}%
}
\caption{Server-Side Backend APIs}
\label{tab:apis}
\end{table*}

We implement our server-side APIs with Flask. We provide three groups of APIs to support the user interaction.

\subsubsection*{Model Preparation API}
The model preparation API provides the front-end interface with necessary model information before running the model. Specifically, the API returns the available model checkpoints, video keys. We are planned to support the user-uploaded video in the future.

\subsubsection*{Model Inference API}
The model inference API takes the two query words, one video id string and one model checkpoint id. The API will returns the results of the intent-network (intent probability) and scoring-network (shot probability). The calculation of the overall shot probability and the selection of the summary shots are conducted on the front-end.
\subsubsection*{Video Shot Frame API}
Video shot frame API takes a video key and a shot index to return the corresponding frame image of the shot. The shot can have multiple frames, we employ a random strategy to select a frame. The API is designed for selecting the representative samples of the intents.

\subsubsection*{Video Shot GIF API}
Video shot GIF API returns a GIF-formatted shot according to the input video key and shot index. The GIF is clipped from the original video via OpenCV. The API is designed for Preview View in the interface.

\subsubsection*{Quantitative Evaluation API}
Quantitative evaluation API takes a summary to generate the quantitative evaluation result. The evaluation includes F-measure, precision and recall. The API is designed for the user-generated summary.

\subsubsection*{API Table}
We list our APIs in Table \ref{tab:apis} with their HTTP methods, parameters and responses.

\subsection*{User Scenario}
Below, we present a user scenario to demonstrate the interaction between the user and interface as well as the connection between the interface and the back-end server.
Before rendering the webpage, the interface will first send a request to Model Preparation API to get the necessary information for the initial view. Then the initial view will be presented to the user.
The user can first input the query words, video, and model checkpoint in the initial view. Here the user inputs the "Food" and "Room" as the words. Then the user chooses the Video-3 and model "default". After submitting the query information, the interface will send a GET request to Model Inference API and render the whole page based on the response. 
We employ an asynchronous rendering mechanism to reduce the latency. The asynchronous mechanism allows the interface to first renders the Summary View and Intent View before rendering the representative frames and Quantitative Evaluation View. During the process, the interface selects the representative samples based on the shot selection probability (shot score) and requests the Video Shot Frame API to get the corresponding image. It also sends the generated summary to Quantitative Evaluation API to render the Evaluation View. 
After rendering all the views, the user can brush on the overview bar chart and the brush operation will determinate the temporal range in the focus bar chart. The user can view different intents and understand them by the representative samples. Then the user can adjust the intent probability based on his preference. The adjusted probability distribution will generate a new summary, which will change the Summary View and Quantitative View. To get the new evaluation result, the interface sends a request to Quantitative Evaluation API again. 
To view the specific shot, the user can hover on the shot. The operation will make the interface send a request to Video Shot GIF API, whose response will be rendered in Preview View.

\begin{figure*}[!h]
\centering
\includegraphics[trim=0 0 0 0,clip, width=1\textwidth]{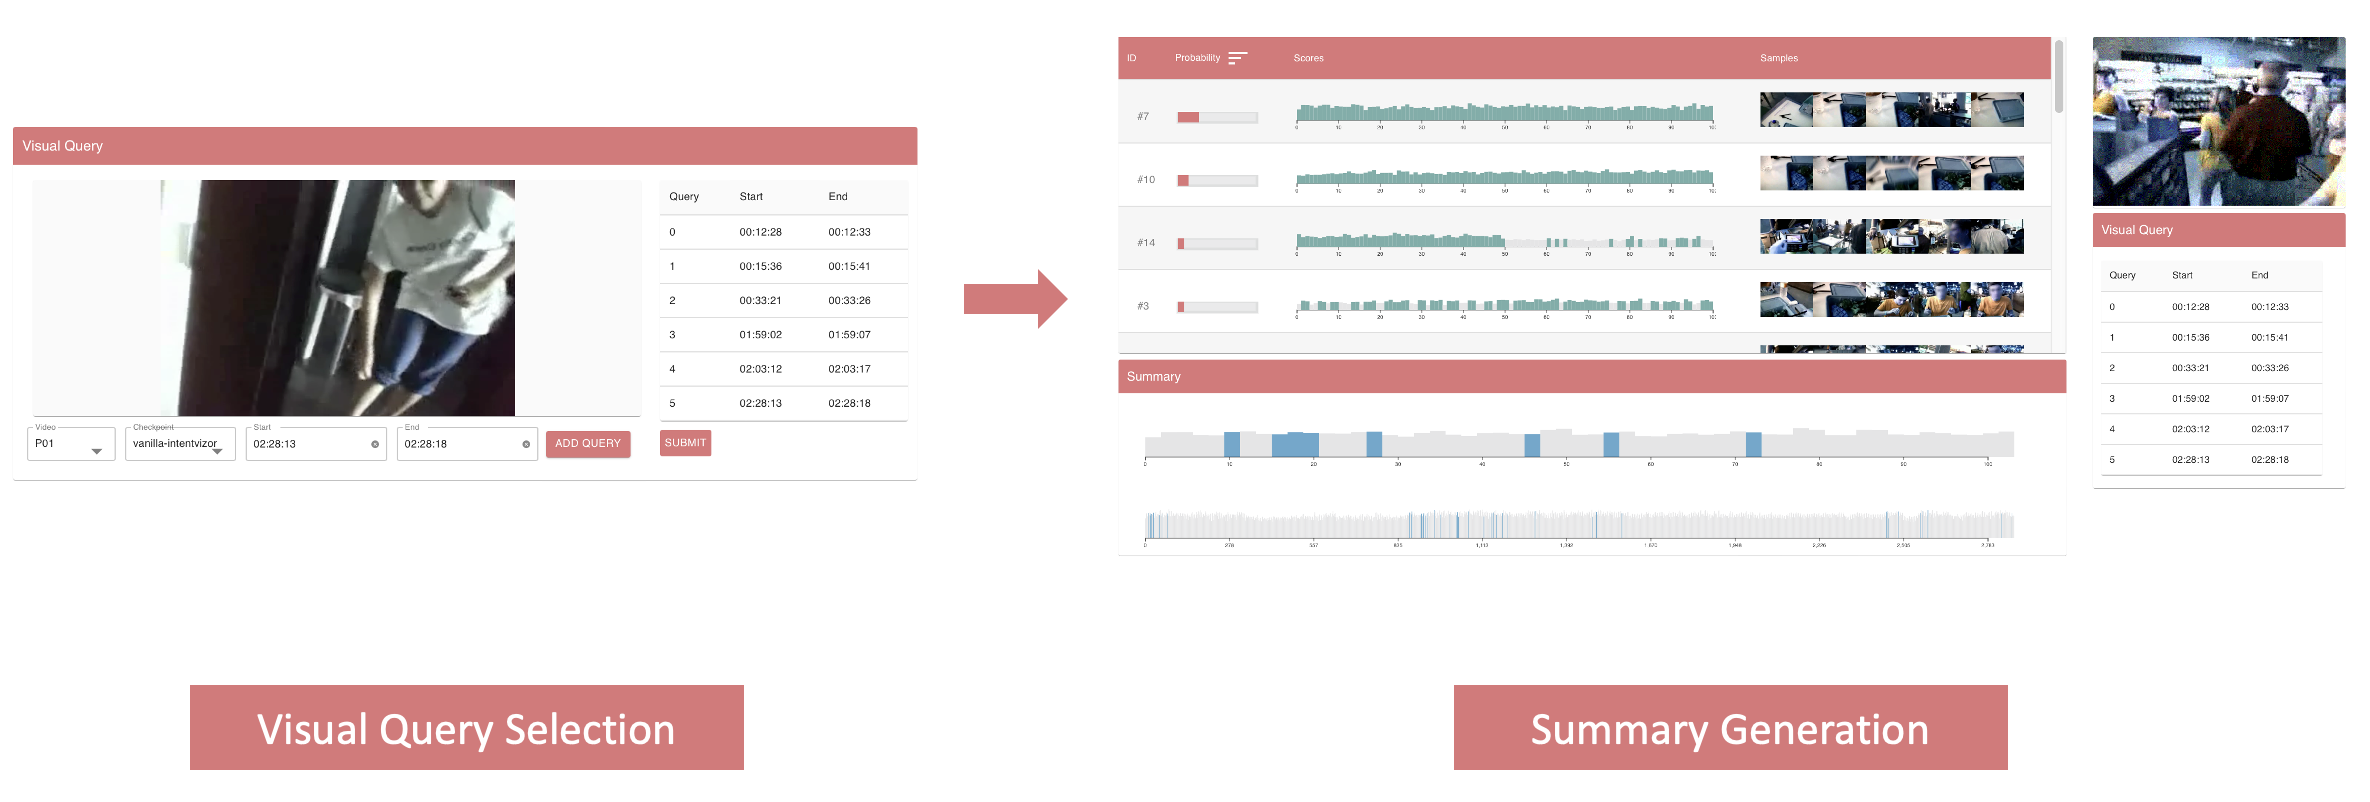} % Reduce the figure size so that it is slightly narrower than the column. Don't use precise values for figure width.This setup will avoid overfull boxes.
\caption{The prototype snapshot for the visual-query based video summarization. There are two pages for the user. Firstly, \textbf{Visual Query Selection} page allows the user selects the query shots based on the input video. The query shots are specified based on the user-inputted start and end times. Then, \textbf{Summary Generation} page renders the generated summaries and supports the user interaction in a way similar to the textual-query prototype.}
\label{fig:visual-query-prototype}
\end{figure*}

We also implement a prototype for the visual-query task as shown in Fig. \ref{fig:visual-query-prototype}. The user can select a series of video shots based on the start and end times. 
Such a method allows the user to flexibly choose the queries and enhances the generalization ability of the method. 
After the user finish the query setting, the interface can send the user queries to the backend server, which predicts the user intents and the initial video summary. Then, the front-end interface renders the response and supports the user interaction, similar to the textual-query prototype.
