# Supplementary material for: IntentVizor: Towards Generic Query Guided Interactive Video Summarization
Source: arXiv:2109.14834 source file (2022-03-29)
Supplement: Supplementary file 3 [file visual.tex]

\section*{Appendix A: Visual Query Dataset}
\begin{algorithm}
\caption{Visual Query Generation}\label{alg:visual}
\begin{algorithmic}
\Require $\boldsymbol{A} = \{\alpha_1, \alpha_2, \alpha_T  \}$ as the sequence of the shot's semantic tags
\Require $\boldsymbol{S} = \{s_1, s_2, s_P  \}$ as the summary shots of the video
\Require $k$ as the target visual query number
\Ensure $Q$ as set of representative query shots in $S$.
\State $W \gets Matrix(P, P)$
\State {$i=0$}
\While{$i<P$ }
\State {$j=0$}
\While{$j<P$ }
\State $W[i,j] = SemanticIOU(s_i, s_j)$
\State{$j \gets j + 1$}
\EndWhile
\State{$i \gets i + 1$}
\EndWhile
\State $G \gets ConstructGraphFromWeights(W) $
% \State $G \gets ConstructGraphFromPairwiseDistance(M) $
\State $D \gets EigenVectorCentrality(G)$
\State $S' \gets RankByCentrality(S,D)$
\State $Q \gets S'[:k]$
\end{algorithmic}
\end{algorithm}

In this appendix, we present the details of our proposed visual query dataset.
We build our visual-query dataset on the text-query dataset. For each annotated summarization, we employ the eigenvector centrality as the criteria to pick the most representative shots as the query shots. 
\subsection*{Query Generation}
We employ eigenvector-centrality method to select the most representative shots as the query shots. We detail our query generation in Algorithm \ref{alg:visual}. For each video summary set $S$, we first compute the pairwise semantic IOU \cite{sharghi_query-focused_2017} of the shots in the summary set $S$. In order to do it, we first create a zero-valued matrix $W$ of $P \times P$. Then we loop over the summary set to compute the semantic IOU between every pair of the shots. 
The function $SemanticIOU$ follows the implementation of \cite{sharghi_query-focused_2017}.
The result will be stored in the matrix $W$.
Then, we build a weighted undirected graph $G$ based on the obtained IOU weight matrix $W$. We implement the function $ConstructWeightedGraph$ to fulfill it. Then, we can compute the eigen-vector centrality of each vertex by a Python package called Networkx. We wrap their implementation in the function $EigenVectorCentrality$, which outputs a dictionary $D$ for the eigen-vector centrality values of the all shots.
Finally, we can rank the vertices by the eigen-vector centrality and pick the top-k as the query shots. We implement a function $RankByCentrality$ to fulfill it. The result of the function is a ranked list $S'$ of the shots in $S$.
In practice, we set $k=5$.

\subsection*{Dataset Examples}
We present some samples in the dataset as follows. Specifically, we put the visual query on top of the full video summary as shown in Figure 1-4. The four examples are collected from the four different videos. 

Figure \ref{fig:p01} shows the visual query and summary for Video-1 when the query words are ``Food" and ``Men". We can find the five visual queries include the scenarios when a man is eating the food, which follows the textual query and are close to the full summary. 

Similarly, we can find that in Figure \ref{fig:p02}, the visual summary also follows both the textual query and the full video summary. The query words are ``Garden" and ``Party". We can find that the query shot \#1, \#3, \#4, \#5 are all related to the ``Garden" while the query shot \#3 and \#5 are related to ``Party". We notice that the query \#2 is a car driving scenario, which is not related to either ``Party" or ``Garden". However, by checking the full video summary, we find that there are a lot of car driving scenarios in the full video summary. Thus, the query shot \#2 is closely related to the full video summary.

In Figure \ref{fig:p03}, the query words are ``Hands" and ``Room". We find that the query \#2, \#3 and \#4 have a hand in the picture, while all of the query shots are captured in a room.

In Figure \ref{fig:p04}, the query words are ``Sun" and ``Tree", we find that the queries are taken on the sunny day, which relates to the query word ``Sun". Also, the query shot \#1, \#2, \#4 and \#5 have the trees in the foreground.

\begin{figure*}
\begin{center}
    \begin{tabular}{c}
  \includegraphics[width=0.9 \textwidth]{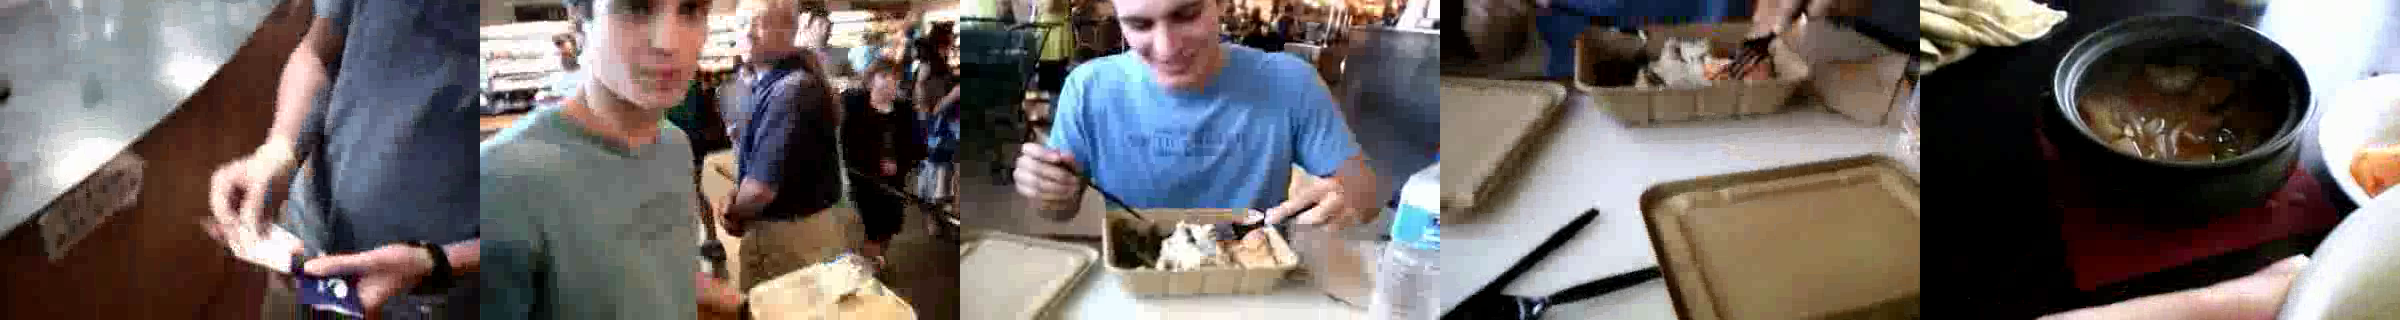}  \\
 Visual Query \\
 \includegraphics[width=0.9 \textwidth]{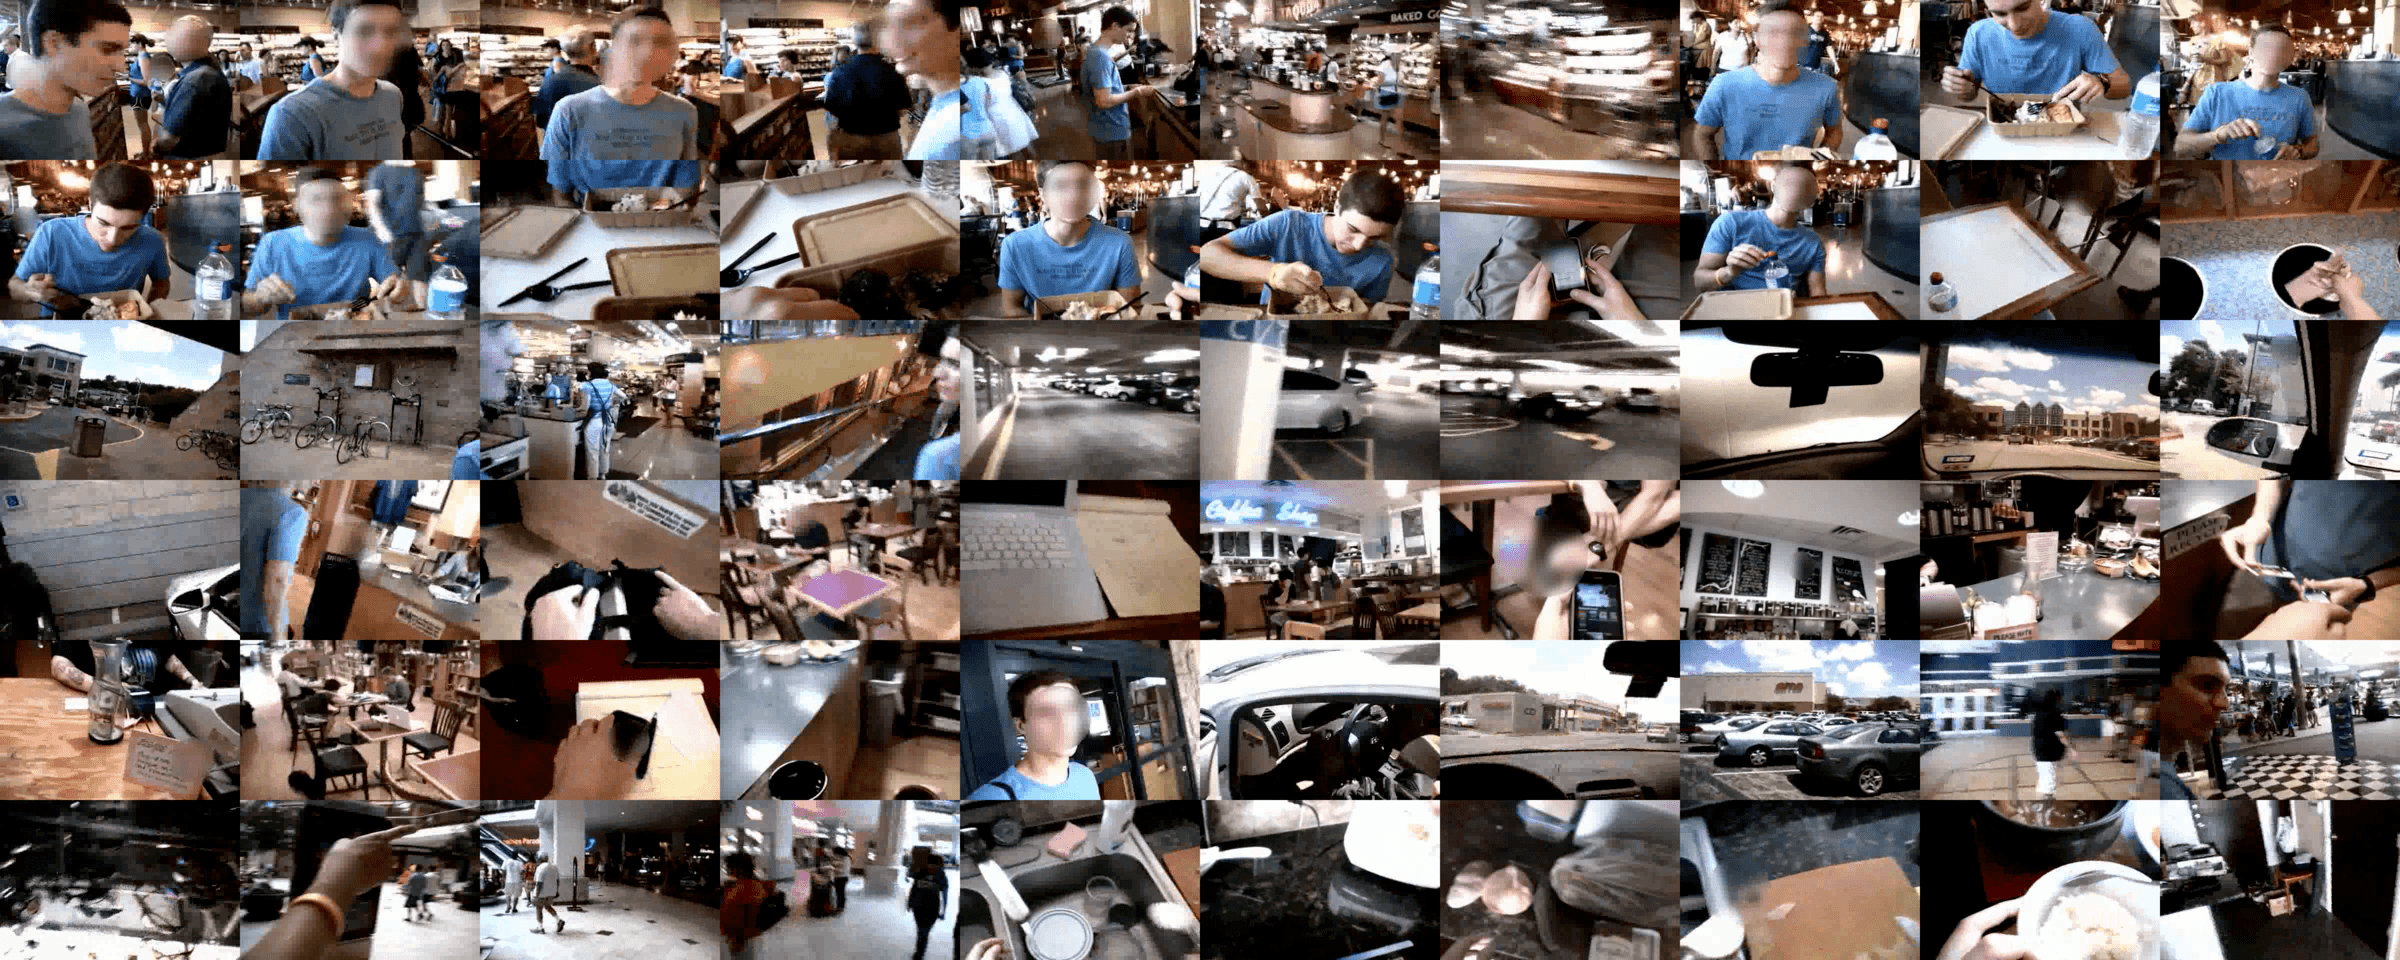} \\ Full Video Summary \\

\end{tabular}

\end{center}
\caption{``Food" and ``Men" on Video 1}
\label{fig:p01}
\end{figure*}

\begin{figure*}
\begin{center}
    \begin{tabular}{c}
  \includegraphics[width=0.9 \textwidth]{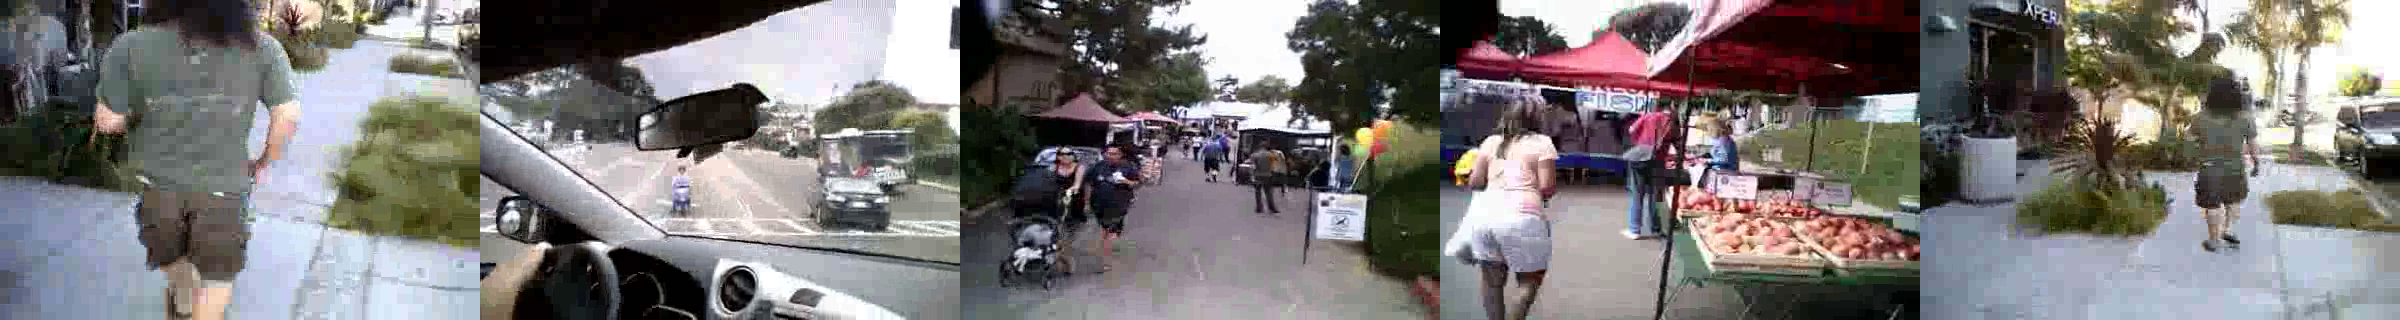}  \\
 Visual Query \\
 \includegraphics[width=0.9 \textwidth]{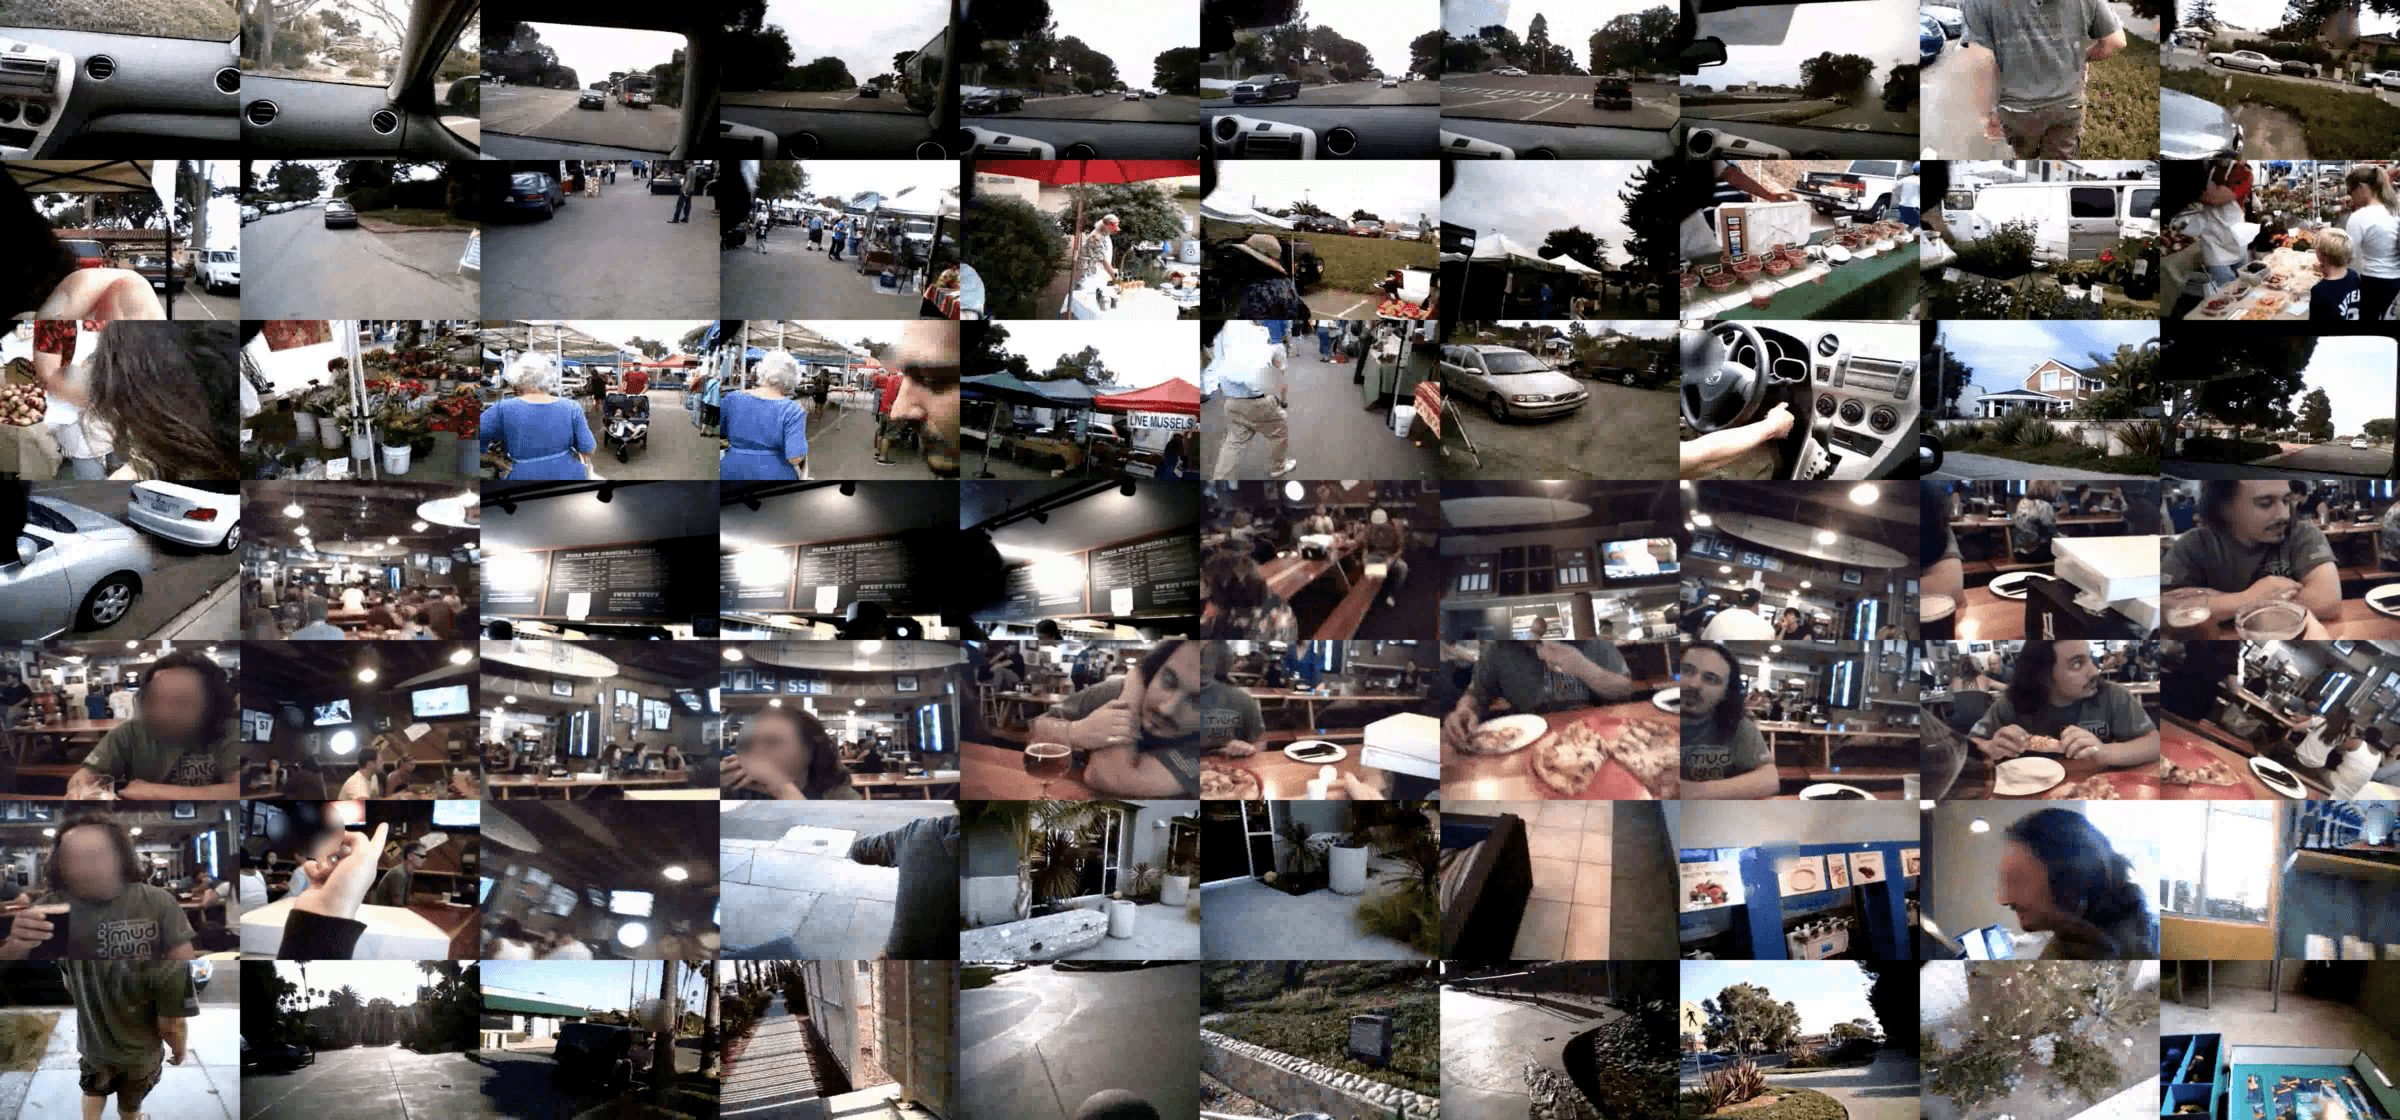} \\ Full Video Summary \\

\end{tabular}

\end{center}
\caption{``Garden" and ``Party" on Video 2}
\label{fig:p02}
\end{figure*}

\begin{figure*}
\begin{center}
    \begin{tabular}{c}
  \includegraphics[width=0.9 \textwidth]{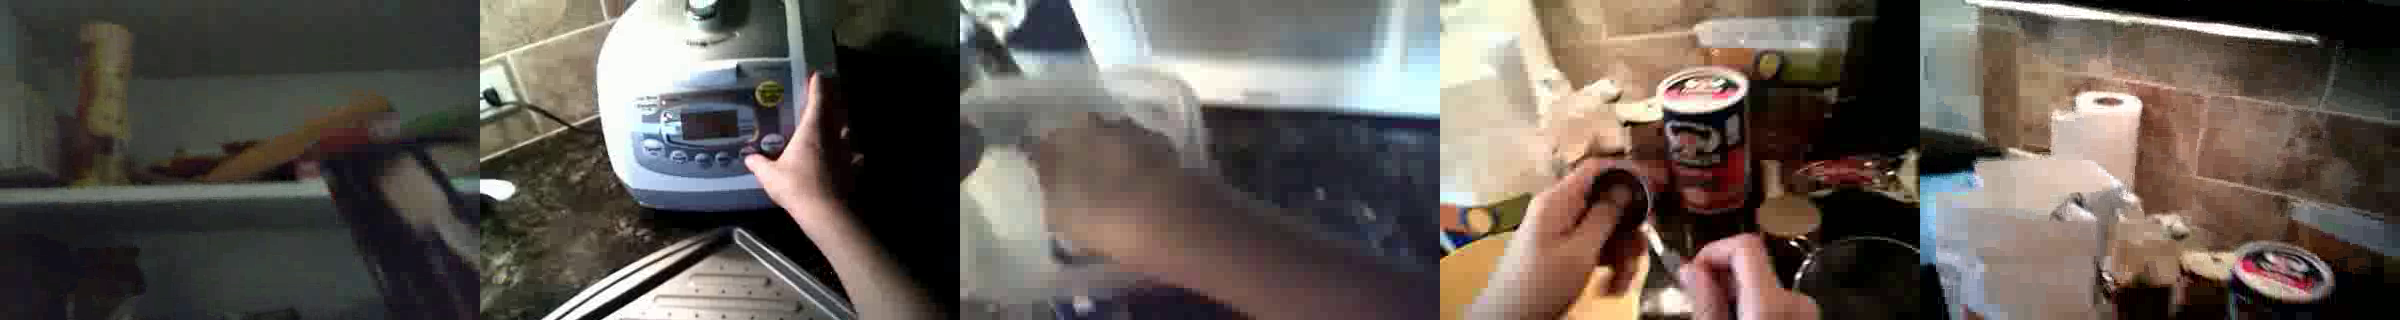}  \\
 Visual Query \\
 \includegraphics[width=0.9 \textwidth]{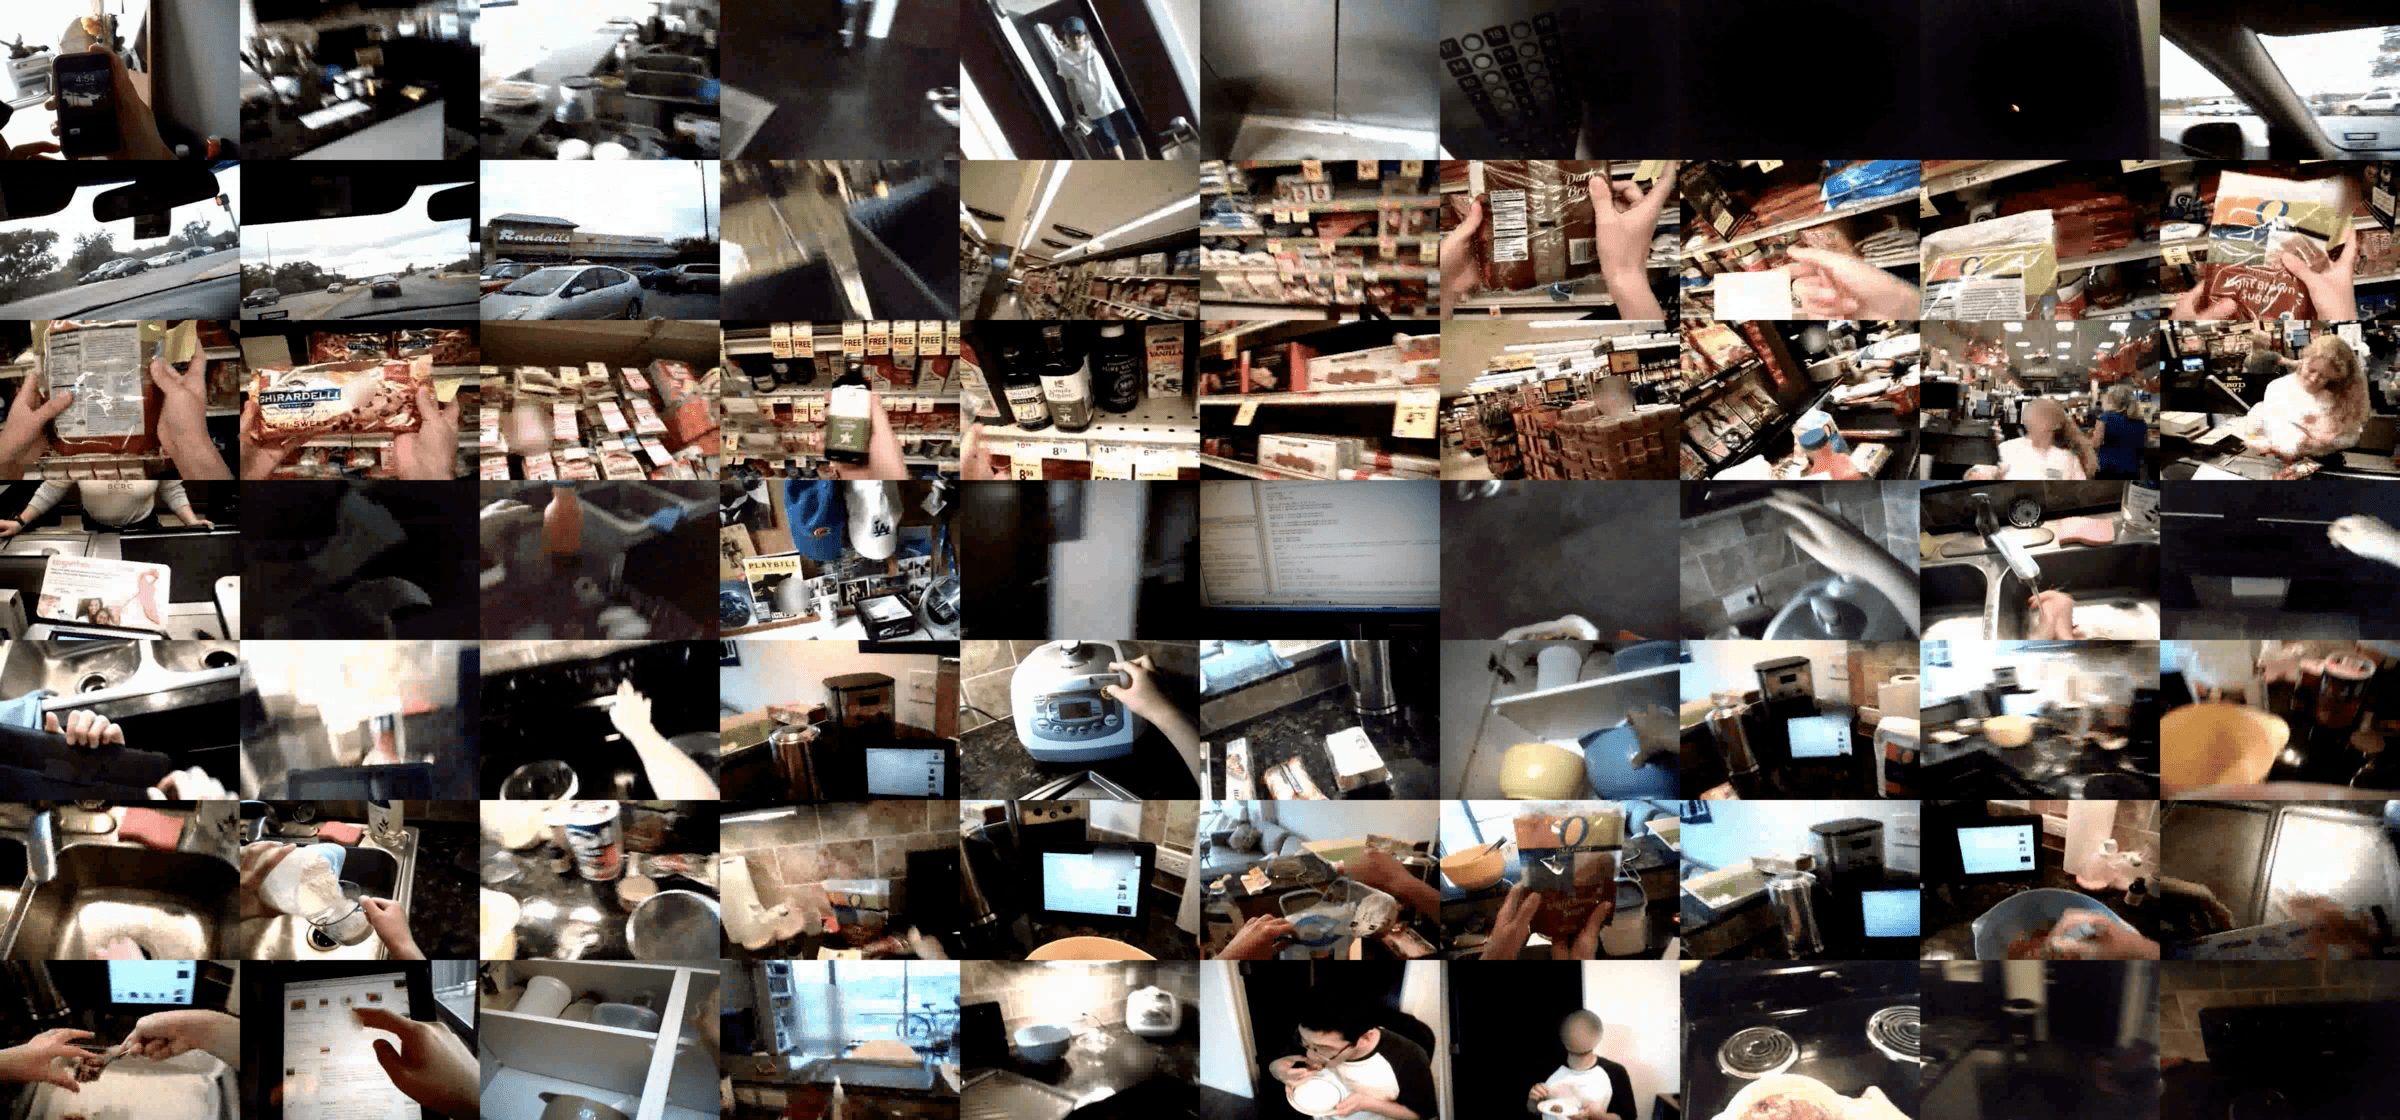} \\ Full Video Summary \\

\end{tabular}

\end{center}
\caption{``Hands" and ``Room" on Video 3}
\label{fig:p03}
\end{figure*}

\begin{figure*}
\begin{center}
    \begin{tabular}{c}
  \includegraphics[width=0.9 \textwidth]{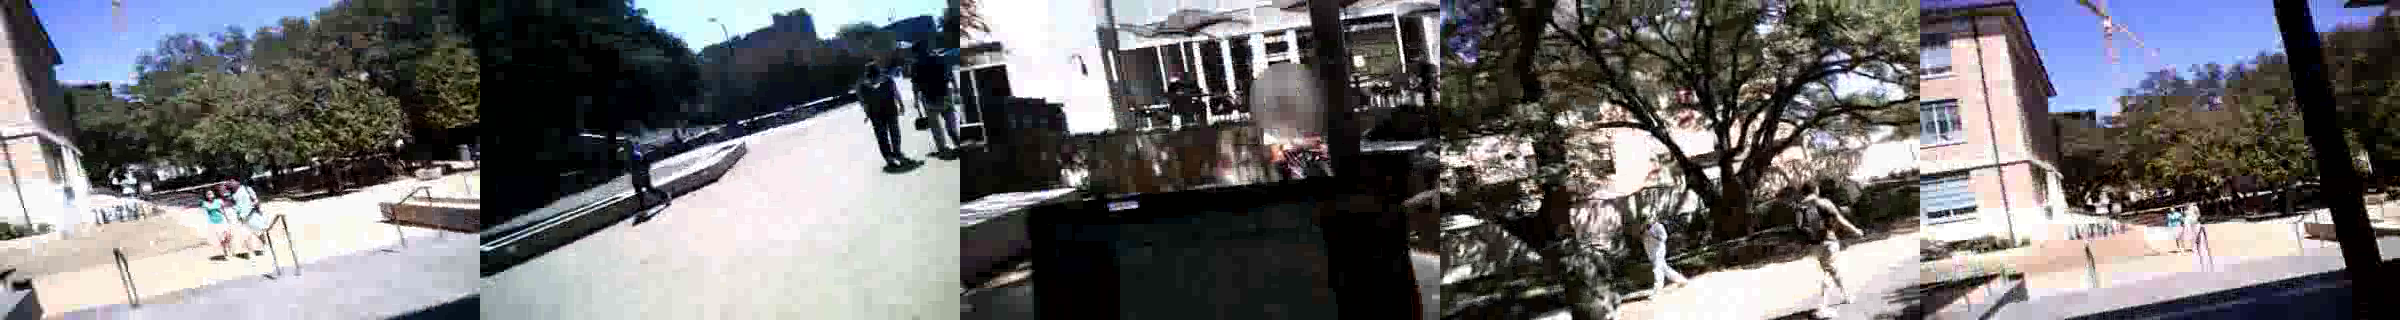}  \\
 Visual Query \\
 \includegraphics[width=0.9 \textwidth]{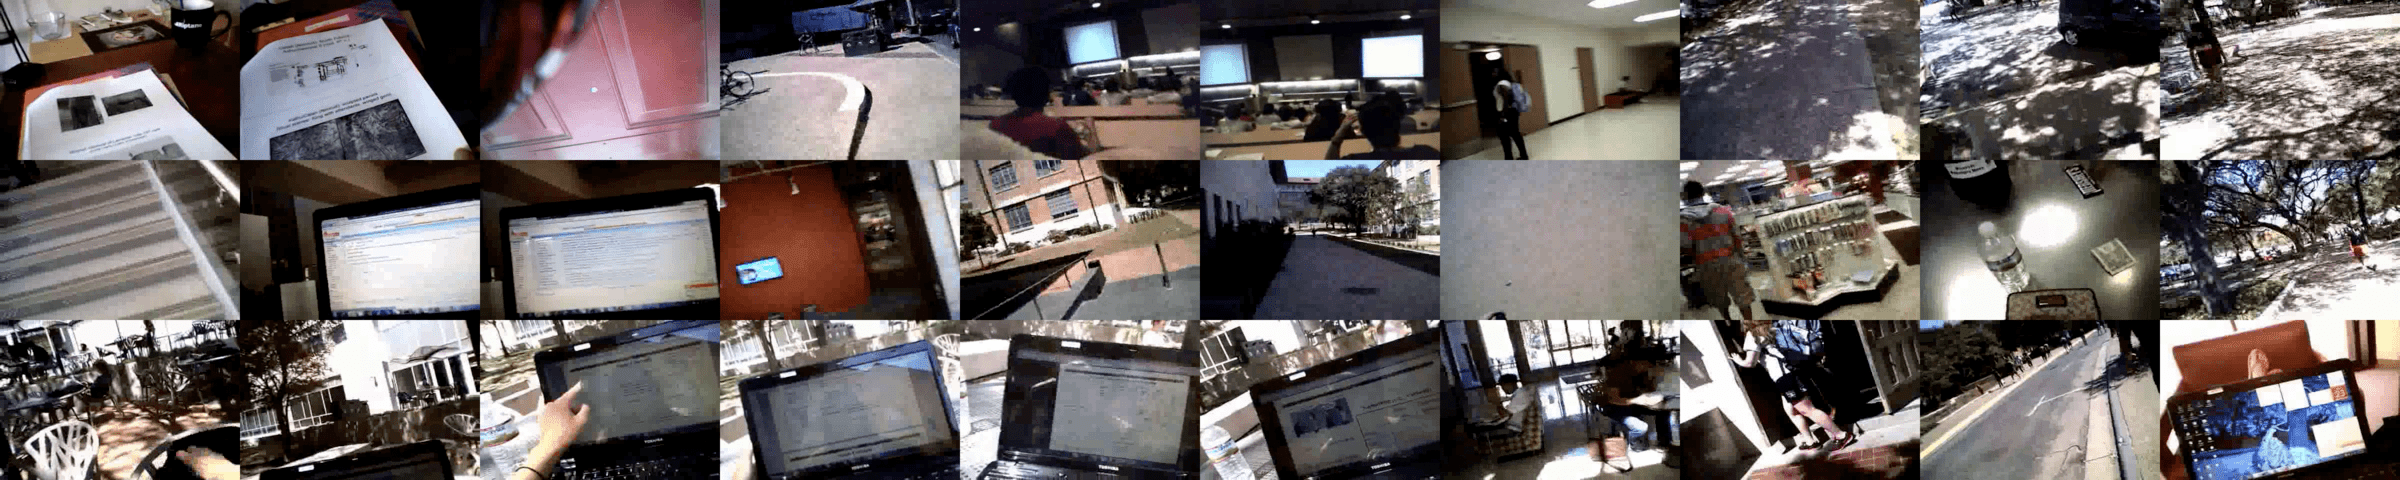} \\ Full Video Summary \\

\end{tabular}

\end{center}
\caption{``Sun" and ``Tree" on Video 4}
\label{fig:p04}
\end{figure*}
