# Supplementary material for: IntentVizor: Towards Generic Query Guided Interactive Video Summarization
Source: arXiv:2109.14834 source file (2022-03-29)
Supplement: Supplementary file 4 [file experiments.tex]

\section*{Appendix D: Full Experiment Result}

In this appendix, we present the full experiment results of the ablation study in Table \ref{tab:full-exp}. We group the methods based on the dataset and the belonging study. We also compute the standard deviation for each method.
